# Supplementary material for: Large quality factor in sheet metamaterials made from dark dielectric meta-atoms
Source: arXiv:1405.7915 source file (2014-05-30)
Supplement: Supplementary file 1 [file SupplMat_DielectricMetaAtoms_rev.pdf]

# Supplemental Material to "Large quality factor in sheet metamaterials made from dark dielectric meta-atoms"

Aditya Jain,[1] Philippe Tassin,[1,*] Thomas Koschny,[1] and Costas M. Soukoulis[1,2]

[1]*Ames Laboratory—U.S. DOE and Department of Physics and Astronomy, Iowa State University, Ames, Iowa 50011, USA*

[2]*Institute of Electronic Structure and Lasers (IESL), FORTH, 71110 Heraklion, Crete, Greece*

(Dated: November 15, 2013)

## METHODS

### Experiments

The alumina substrate was placed in the custom-built fixture depicted in Fig. S8. The fixture is mounted between the flanges of two X band waveguides that are connected to an HP E8364 vector network analyzer. The receiver signals were manually corrected for imperfect-switch effects and were calibrated using a TRM method based on an 8-term error model. The remaining systematic error is smaller than 1% (determined through the measurement of calibration standards)—random noise is reduced below 1% by statistical averaging. The fixture has a twofold purpose:

1. It allows mounting an alumina slab larger than the cross-section of the WR-90 rectangular waveguide, so that the bound states are defined by the edges of the mechanical-precision waveguides rather than by the size of a cut-out alumina slab. Our simulations demonstrate that the field of the bound state decays faster than 20 dB/mm in the gap between the waveguide flanges. The alumina slab is in turn surrounded by a steel frame to prevent leakage of energy from the fundamental waveguide mode and to avoid the existence of TEM modes circulating in the parallel-plate waveguide formed by the gap between the flanges (the steel frame is small enough so that the first TEM mode lies above the X band).

2. By mounting the fixture between spring loads and micrometer screw gauges, we have complete control over the positioning of the sample. In addition, they enable to move the sample horizontally in the waveguide, i.e., the setup acts as a micrometer stage.

### Simulations

All computer simulations are performed using CST Microwave Studio, an electromagnetics solver using the finite-integration method. Input parameters are the geometry which is measured and/or taken from mechanical specifications. Copper (for the wire as well as for WR-90 waveguide) is modelled as a metal with conductivity $5.8 \times 10^7$ S/m, and the permittivity of alumina was determined by fitting to the experimental results. Excellent agreement with the experimental spectra (compare results from experiments and simulations in Fig. S4, in Fig. S5, and Fig. S6) is obtained for $\varepsilon_{\text{alumina}} = 9.71$ with a loss tangent of $6.8 \times 10^{-4}$, which agrees with the manufacturer's specification. The eigenstates of the alumina slab (Fig. 1), the electric dipole mode of the cut wire (Fig. 2) and the results for the negative-permittivity metamaterial (Fig. 3) and the negative-permeability metamaterial (Fig. 6) were obtained from simulations of an alumina slab in a plain WR-90 waveguide with copper edges. All results concerning the dispersion-engineered metamaterial (Fig. 4, Fig. 5, Fig. S4, Fig. S5, and Fig. S5) were obtained from a full implementation of the alumina slab in the custom-built fixture as described above. The numerical results in Fig. 5 were experimentally validated for the shortest and longest wire and the results shown in Fig. S6 demonstrate that the results from the computer simulations are in excellent agreement with the results from the experiments.

### Effective permittivity and permeability

The effective permittivity and permeability of the metamaterials was determined using the method of Smith *et al.* [1, 2]. The thickness of the equivalent slab of homogeneous material was taken the same as the thickness of the alumina slab. The retrieval method was adapted to account for the specific dispersion of the fundamental mode in the WR-90 waveguide, i.e., the standard retrieval method returns the wavenumber in the propagation direction $k_\perp$ and the waveguide impedance $\xi$ of the effective medium. The effective permittivity and permeability can then be obtained from

$$\mu = \frac{k_\perp}{k_0} \frac{\xi}{\sqrt{1 - \left(k_{//}/k_0\right)^2}}, \tag{1}$$

$$\varepsilon = \frac{\sqrt{1 - \left(k_{//}/k_0\right)^2}}{\xi} \left( \frac{k_\perp}{k_0} + \frac{k_{//}^2}{k_0 k_\perp} \right), \tag{2}$$

where $k_0 = \omega/c$ is the free-space wavenumber and $k_{//} = \pi/a$ is the transverse wavenumber of the fundamental waveguide mode.

Work at Ames Lab was partially supported by the U.S. Dept. of Energy, Basic Energy Science, Materials Sciences and Engineering, Contract No. DE-AC02-07CH11358 (experiments), and by the U.S. Office of Naval Research, Award No. N00014-10-1-0925 (theory).

---

* Present address: Department of Applied Physics, Chalmers University, SE-412 96 Göteborg, Sweden

[1] D. R. Smith, S. Schultz, P. Markos, and C. M. Soukoulis, Phys. Rev. B **65**, 195104 (2002).
[2] D. R. Smith, D. C. Vier, T. Koschny, and C. M. Soukoulis, Phys. Rev. E **71**, 036617 (2005).

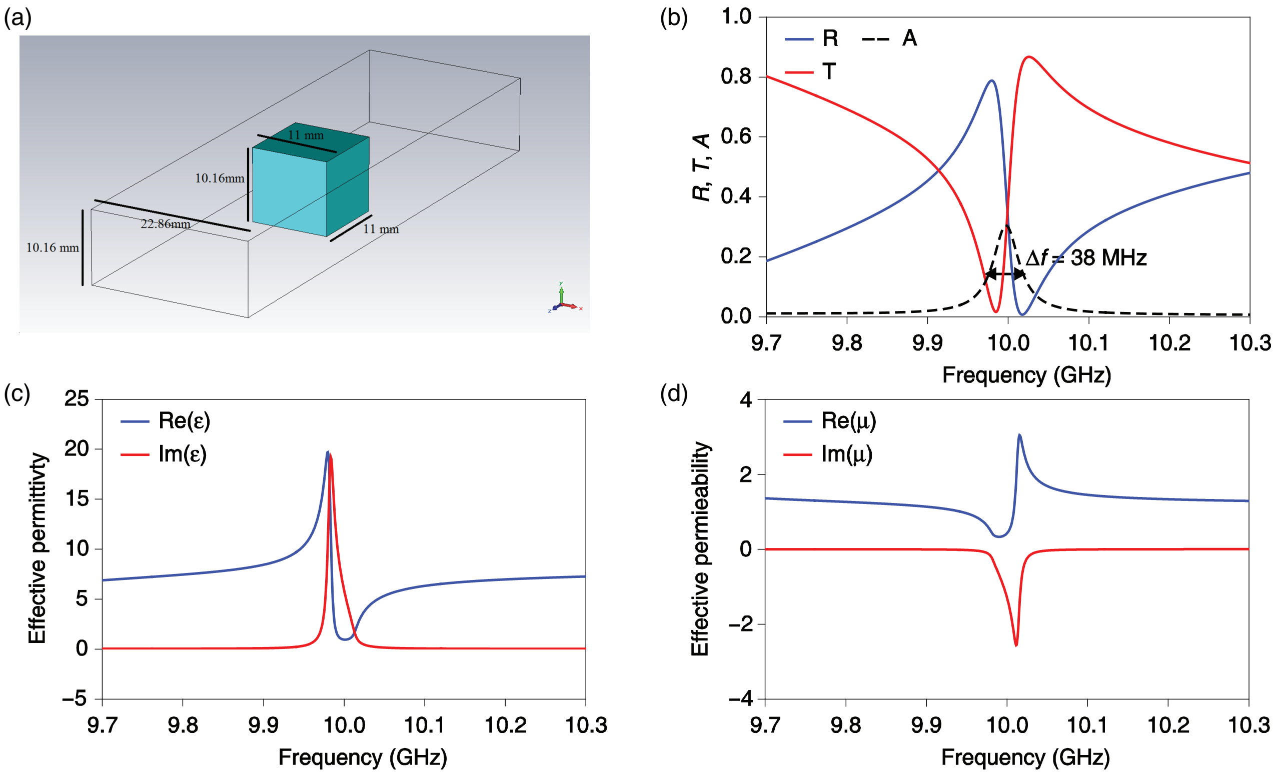


FIG. S1: Scattering on a Mie-dielectric-particle metamaterial. The quality factor is large ($Q = 263$), but there are strong periodicity artefacts (cut-off of the permittivity resonance and strong anti-resonance in the permeability). (a) The metamaterial made of dielectric square-based cylindrical particles. (b) Reflectance, transmittance, and absorbance. (c) Retrieved effective permittivity derived from the scattering data. (d) Retrieved effective permeability derived from the scattering data.

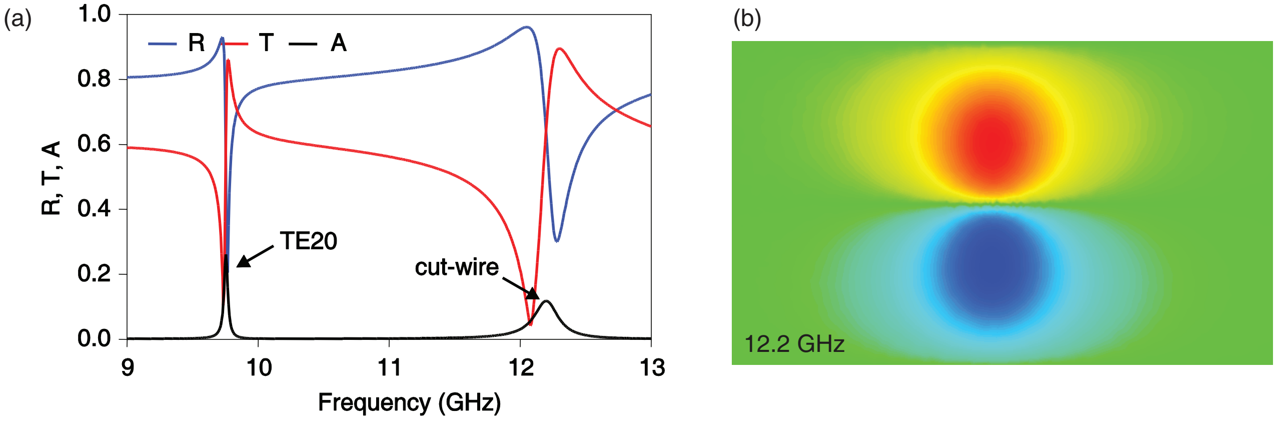


FIG. S2: (a) Scattering parameters and absorption of the dielectric metamaterial with a cut wire as nonresonant scatterer. The narrow, high-quality resonance at 9.74 GHz is the dark state in the dielectric meta-atom. The resonance at 12.2 GHz is the electric-dipole resonance of the cut wire (it is far away from the dark-state resonance, i.e., we use the cut wire as a nonresonant scatterer). (b) Electric field plot at the 12.2 GHz resonance. The electric dipole field can be easily recognized.

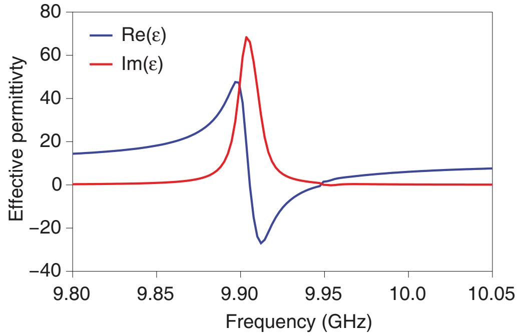


FIG. S3: Effective permittivity obtained from experiments for the dielectric meta-atom decorated with a 6.0-mm-long wire as secondary scatterer displaced over 2 mm from the centre. The experimental results are in good agreement with the simulations presented in Fig. 3 of the main paper.

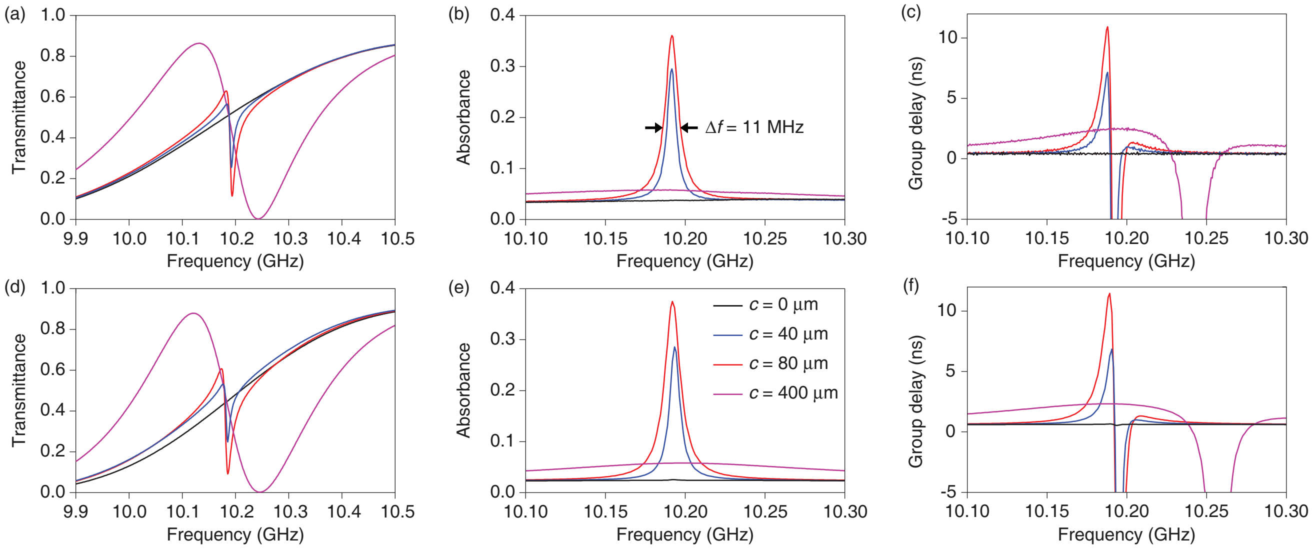


FIG. S4: Transmission, absorbance and group delay of the MM with the dielectric meta-atom and a 7.79-mm-long cut wire as secondary scattering antenna. (a)-(c) Obtained from the experiment. (d)-(f) Obtained from numerical simulations.

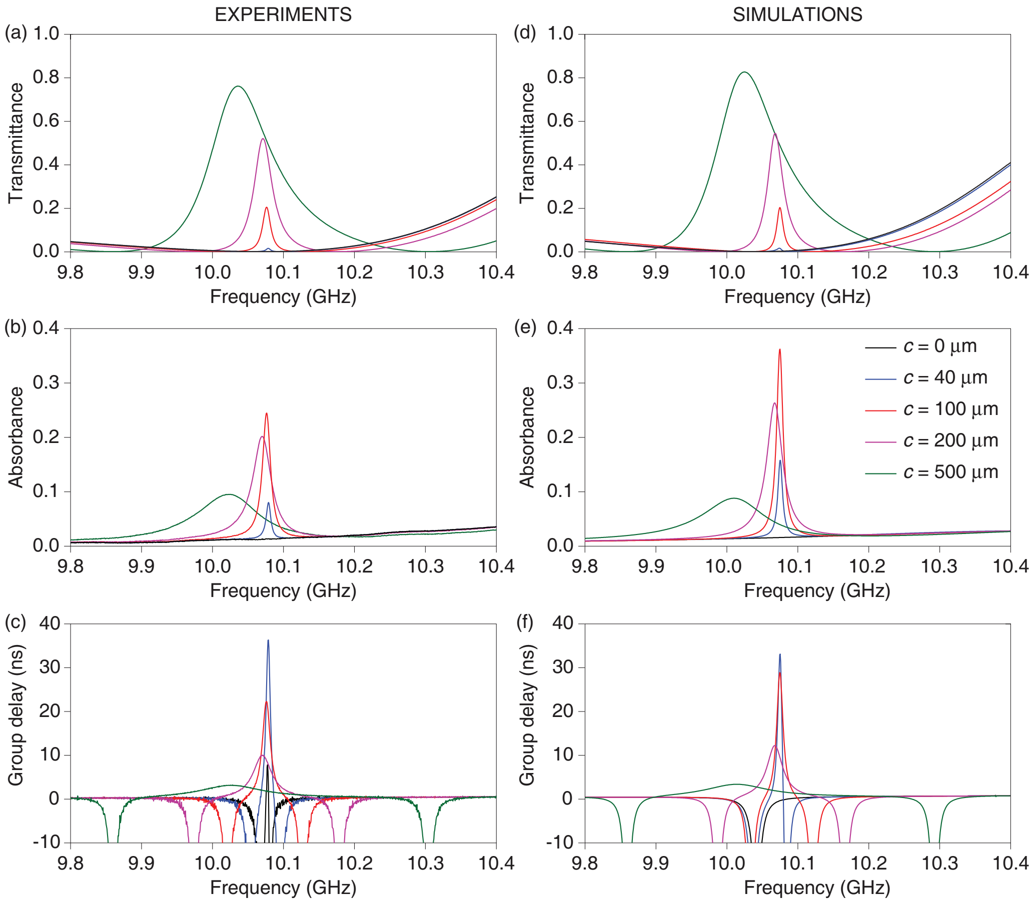


FIG. S5: Transmission, absorbance and group delay of the metamaterial with the dielectric meta-atom and a 7.29-mm-long cut wire as secondary scattering antenna. (a)-(c) Obtained from the experiment. (d)-(f) Obtained from numerical simulations.

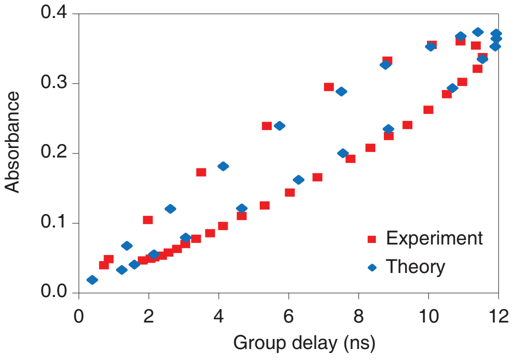


FIG. S6: Absorbance vs. group delay of the dispersion-engineered metamaterial with the cut-wire antenna of length $L = 7.79$ mm.

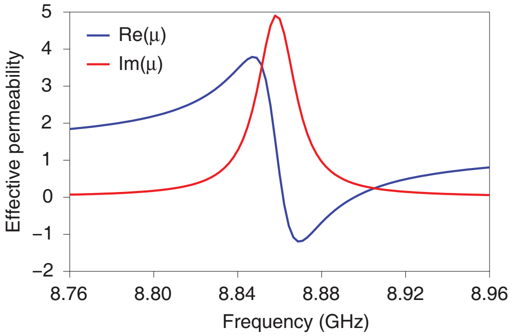


FIG. S7: Effective permeability obtained from experiments for the dielectric meta-atom decorated with a 7-mm-long cut-wire pair as secondary scatterer. The experimental results are in good agreement with the simulations presented in Fig. 6(b) of the main paper.

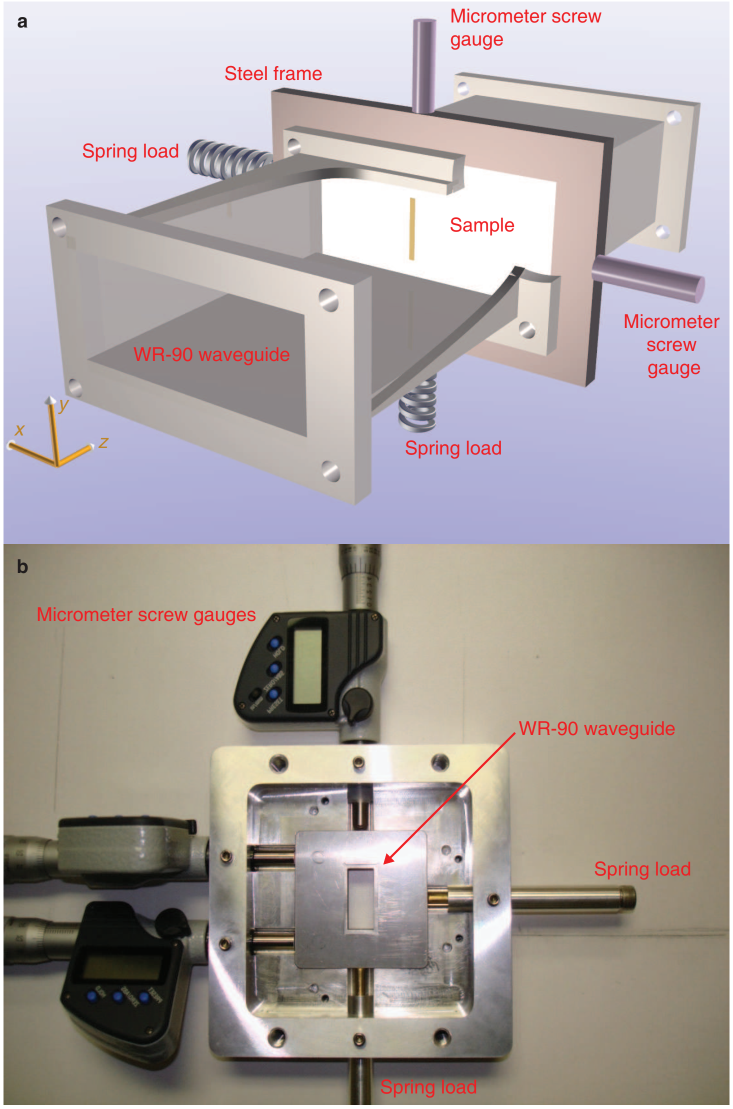


FIG. S8: The experimental setup with the custom-built fixture. (a) Perspective view. (b) Side view.
